# Supplementary material for: FireRedTTS: A Foundation Text-To-Speech Framework for Industry-Level Generative Speech Applications
Source: arXiv:2409.03283 source file (2025-04-11)
Supplement: Supplementary file 1 [file appendix.tex]

\begin{center}{\bf {\LARGE Appendices} }
\end{center}

\section{Details of Data Processing Pipeline} \label{appendix:dataloader}

\subsection{VAD}
\begin{table}[!ht]
\centering
\begin{tabular}{cccc}
\hline
 & \textbf{Accuracy($\uparrow$)} & \textbf{F1($\uparrow$)} & \textbf{RTF($\downarrow$)} \\ \hline \hline
\textbf{Red VAD} & \textbf{0.888} & \textbf{0.920} & 0.0066 \\
FunASR VAD & 0.811 & 0.863 & 0.0163 \\ \hline
\end{tabular}
\caption{Comparison between RedVAD, FunASR VAD, and PyDub VAD in terms of accuracy, F1 score and real-time-factor(RTF).}
\label{tab:vad_compare}
\end{table}

\subsection{ASR}
\begin{table}[!ht]
\centering
\begin{tabular}{cccc}
\hline
 & \textbf{Video($\downarrow$)} & \textbf{Live($\downarrow$)} & \textbf{Message($\downarrow$)} \\ \hline \hline
\textbf{RedASR} & \textbf{5.5} & \textbf{4.8} & \textbf{6.9} \\
FunASR & 8.7 & 6.5 & 7.9 \\ \hline
\end{tabular}
\caption{Comparison of transcription WER between RedASR and publicly available FunASR across three different speech sources.}
\label{tab:asr_compare}
\end{table}

\subsection{Pipeline Statistics}
\begin{table}[!ht]
\centering
\begin{tabular}{ccc}
\hline
 & \textbf{Total Duration(h)} & \textbf{Remain(\%)} \\ \hline \hline
Original & 260.3k & 100\% \\ \hline
Enhancement & 260.3k & 100\% \\
VAD & 245.2k & 94.22\% \\
Speaker Clustering & 220.9k & 84.88\% \\
Quality Filtering & 111.8k & 42.95\% \\ \hline
\end{tabular}
\caption{Amount of speech data remaining after each processing step.}
\label{tab:pipeline_funnel}
\end{table}

\section{Triple-Dataloader} \label{appendix:dataloader}
\subsection{Model structure}
